# Supplementary material for: When MOE Meets LLMs: Parameter Efficient Fine-tuning for Multi-task Medical Applications
Source: arXiv:2310.18339 source file (2024-05-31)
Supplement: Supplementary file 1 [file 7Appendix.tex]

%%% Hyper-parameter Setting %%%
\begin{table*}[]
\centering
\caption{The hyper-parameter settings in our experiments.}
\begin{tabular}{lccccc}
\toprule
Hyper-parameters & P-Tuning & LoRA (Full) & LoRA (Single) & LoRA (Full+TP) & MOELoRA \\ 
\midrule
Batch Size & 64 & 64 & 64 & 64 & 64 \\
Learning Rate & 2e-4 & 2e-4 & 2e-4 & 2e-4 & 2e-4 \\
Max Steps & 8,000 & 8,000 & 800 & 8,000 & 8,000 \\
Max Input Length & 1,024 & 1,024 & 1,024 & 1,024 & 1,024 \\
Max Output Length & 196 & 196 & 196 & 196 & 196 \\
Training Precision & FP16 & FP16 & FP16 & FP16 & FP16 \\
Temperature & 0.95 & 0.95 & 0.95 & 0.95 & 0.95 \\
Prompt Sequence Length & 128 & - & - & - & - \\
LoRA Rank & - & 16 & 8 & 16 & 16 \\
Task Embedding & - & - & - & - & 64 \\
Expert Number & - & - & - & - & 16 \\ 
\bottomrule
\end{tabular}
\label{tab:exp_hyper}
\end{table*}
%%% Hyper-parameter Setting %%%

\section{Experimental Settings}

In this section, we will describe some settings of our experiments in detail, including baselines and their implementations, implementation details and evaluation metrics.

\subsection{Baselines and Implementation} \label{sec:appendix_baseline}
In the experiments, two LLMs without fine-tuned baselines are compared, \ie ChatGPT~\cite{brown2020language} and Huatuo~\cite{wang2023huatuo}. In comparison, we utilize in-context learning to prompt the model to complete corresponding medical tasks. The brief introduction and implementation are illustrated as follows:
\begin{itemize}[leftmargin=*]
    \item \textbf{ChatGPT}~\cite{brown2020language}. ChatGPT is one of the most popular LLMs that contains over 100 billion parameters. It is pre-trained on a large corpus of various data, which imbues it with the potential to complete medical tasks. To inspire task-relevant ability, we adopt in-context learning when comparing. In detail, for each task, we randomly sample $3$ to $10$ input-output pairs from the training data of this task to organize the demonstration. The sampled number is based on the length of demonstration texts, which aims to fill the input length to the maximum.

    \item \textbf{Huatuo}~\cite{wang2023huatuo}. Huatuo first constructs a Chinese medical instruction dataset by a medical database. They utilize the instruction dataset to fine-tune several open-sourced LLMs, such as LLaMA-7B~\cite{touvron2023llama} and ChatGLM-6B~\cite{du2022glm}. In our experiment, we use the version of ChatGLM-6B for fair comparison and the same in-context learning method as the ChatGPT baseline.
\end{itemize}

\noindent Besides, based on ChatGLM-6B~\cite{du2022glm}, we conduct two types of parameter efficient fine-tuning methods, \ie LoRA~\cite{hu2021lora} and P-Tuning~\cite{liu2023gpt}. Several variants of LoRA are also conducted.
\begin{itemize}[leftmargin=*]
    \item \textbf{P-Tuning}~\cite{liu2023gpt}. P-Tuning designs a trainable prompt encoder to produce continuous prompt vectors, which are inserted into the input sequence. We implement it by fine-tuning the prompt encoder on the data of all tasks.

    \item \textbf{LoRA (Full)}~\cite{hu2021lora}. LoRA designs two low-rank matrices as the trainable parameters for dense layers while freezing all parameters of pre-trained LLMs. LoRA (Full) trains a unique set of LoRA parameters for all tasks.

    \item \textbf{LoRA (Single)}~\cite{hu2021lora}. We implement LoRA (Single) by separately training LoRA for each task. For the time and resource limitation, we adopt the same set of hyper-parameters for all tasks and select the model according to the best average score.

    \item \textbf{LoRA (Full+TP)}~\cite{hu2021lora}. We add simple task demonstration to input texts, which aims to prompt the LLMs with the distinctions between tasks. As for the implementation, we conduct the same training process as LoRA (Full).
\end{itemize}

\noindent To verify whether the cross-task generalization research can be used for multi-task settings, we modify a most recent work to our experiment, \ie LoRAHub~\cite{huang2023lorahub}.
\begin{itemize}[leftmargin=*]
    \item \textbf{LoRAHub}~\cite{huang2023lorahub}. LoRAHub proposes an assembling method to compose LoRA parameters fine-tuned on source tasks and seek the generalization to unseen target tasks. To adapt the LoRAHub to the multi-task setting, we first LoRA fine-tune each task. Then, use the validation of one specified task to learn the composing weight and test the performance for this task. All eight tasks are conducted by the same process.
\end{itemize}

\subsection{Implementation Details} \label{sec:appendix_implementation}
In this section, we introduce the implementation and hyper-parameter details. To ensure the robustness and reproducibility of our results, tests are run thrice by random seeds $\{42,43,44\}$, with average scores reported. 
Since the LoRA fine-tuning for ChatGLM-6B is still highly time-consuming, we adopt parallel computation. 
In detail, we utilize the deepspeed package~\cite{rajbhandari2020zero} to distribute the computation on several Tesla V100 GPUs and conduct gradient accumulation for the limited GPU memory. 
With regard to the hyper-parameter setting, we adjust them on the validation dataset.
The detailed hyper-parameter setting of MOELoRA and the baselines with fine-tuning are concluded in Table~\ref{tab:exp_hyper}. 
For LoRAHub, we use the fine-tuned parameters in LoRA (Single) as the source LoRA and adopt hyper-parameters the identical to the original paper. 
In terms of LoRA (Single), we set smaller LoRA rank and max steps to avoid the problem of overfitting. To balance the time and accuracy, we choose the half-precision training, denoted as FP16, for all experiments. Besides, during the testing, we set the temperature as $0.95$ for generation.

%%% Description and Templates for each task %%%
\begin{table*}[!t]
\centering
\caption{The brief description of each task and prompt template examples of the PromptCBLUE dataset.}
\resizebox{1\textwidth}{!}{
\begin{tabular}{c|l|l}
\toprule[1.5pt]
\textbf{Task} & \textbf{Description} & \textbf{Prompt Templates} \\ 
\midrule
\midrule
CMeIE & \makecell[l]{Given the medical texts, recognize the entity pair with required \\ entity relations.} & \makecell[l]{``Please find out the specified entity pairs: [INPUT\_TEXT], the relations need to be \\ recognized:  [LIST\_LABELS]. Answer:''} \\
\midrule
CHIP-CDN & 
\makecell[l]{Given the diagnostic proverbs, require its diagnostic standardized \\ expression, which is selected from ICD-10 dictionary.} & 
\makecell[l]{Give the standardization expression of the following diagnostic proverbs: [INPUT\_TEXT] 
 \\ Candidate set: [LIST\_LABELS]. Note: Select the matching words from ICD-10  diagnosis \\ word candidates. Answer:} \\
\midrule
CHIP-CDEE & 
\makecell[l]{Extract four specific clinical attributes from a report about medical \\ record or medical imaging.} & 
\makecell[l]{Identify the clinical events and their attributes in the sentence [INPUT\_TEXT]. Note: The \\ subject word of the clinical event consists of status, demonstration word and anatomical \\ part. Answer: } \\
\midrule
CHIP-MDCFNPC & 
\makecell[l]{Extract the clinical entities and recognize patient's negatives \\ and positives status on the entity based on a segment \\ of patient-doctor conversation.} & 
\makecell[l]{Please give the negative and positive judgments for the clinical entity in the dialog: [INPUT\_TEXT]. \\ Clinical entity candidate:  [LIST$\_$MENTIONS], Negative and positive options: [LIST$\_$LABELS], \\ Answer:} \\
\midrule
CHIP-CTC & 
Categorize the medical text by clinical test selection criteria. & 
\makecell[l]{[INPUT\_TEXT] What clinical test selection criteria type is this medical text? Type option: [LIST\_LABELS] \\ Answer:} \\
\midrule
KUAKE-QIC & 
Categorize the intent of search query in medical scenarios. & 
\makecell[l]{Identify the intent of the following search query: [INPUT\_TEXT] Option:[LIST\_LABELS] Answer:} \\
\midrule
IMCS-V2-MRG & 
\makecell[l]{Generate the inquiry report according to the dialogue between \\ doctor and patient.} & 
\makecell[l]{Conclude the following inquiry dialogue and give out the inquiry report: [INPUT\_TEXT]. Note: \\ Inquiry report includes query, history of present illness, auxiliary inspection, past medical \\ history, diagnosis and suggestion. Answer: } \\
\midrule
MedDG & 
\makecell[l]{Generate the doctor's next response based on the doctor-patient \\ conversations.} & 
\makecell[l]{Give the doctor's next response based on the following historical dialog conversations: [INPUT\_TEXT] \\ Answer:} \\ 
\bottomrule[1.5pt]
\end{tabular}
\label{tab:appendix_prompt}
}
\end{table*}
%%% Description and Templates for each task %%%

\subsection{Evaluation Metrics} \label{sec:appendix_metrics}

In terms of the evaluation metrics, since different types of tasks are tested, various corresponding evaluation metrics are adopted. Most tasks in our experiments are actually multi-classification problems, so two types of F1 scores are used for these tasks. As for text generation tasks, \ie IMCS-V2-MRG and MedDG, the metric RougeL is applied for evaluation.

\begin{itemize}[leftmargin=*]
    \item \textbf{Micro-F1}. F1-score has been widely used for evaluating multi-classification models. For illustration, we first give some notations for the multi-classification problem. Assume there are $K$ classifications and they are denoted as $\mathcal{S}=\{C_k\}_{k=1}^K$. If the predicted classification is $\hat{C}$ and ground-truth is $\bar{C}$, then each $C_k$ has following measures: $TP_k=|\{\hat{C} = C_k \wedge \bar{C} = C_k \}|$, $FP_k=|\{\hat{C} = C_k \wedge \bar{C} \ne C_k \}|$, $TN_k=|\{\hat{C} \ne C_k \wedge \bar{C} \ne C_k \}|$ and  $FN_k=|\{\hat{C} \ne C_k \wedge \bar{C} = C_k \}|$. According to these measures, we can compute the Micro-F1 values by following formulas:
    \begin{equation}
        {\rm Precision_{micro}} = \frac{\sum_{k=1}^K TP_k}{\sum_{k=1}^K TP_k + \sum_{k=1}^K FP_k} 
    \end{equation}
    \begin{equation}
        {\rm Recall_{micro}} = \frac{\sum_{k=1}^K TP_k}{\sum_{k=1}^K TP_k + \sum_{k=1}^K FN_k} 
    \end{equation}
    \begin{equation}
        {\rm F1_{micro}} = 2 \cdot \frac{{\rm Precision_{micro}} \cdot {\rm Recall_{micro}}}{{\rm Precision_{micro}} + {\rm Recall_{micro}}}
    \end{equation}
    \noindent In our experiments, the task CMeIE, CHIP-CDN, CHIP-CDEE and CHIP-MDCFNPC are evaluated by this metric.

    \item \textbf{Macro-F1}. Compared with Micro-F1, the Macro-F1 metric considers the imbalance between various classifications, so it first averages the precision and recall score before calculating F1. The detailed calculation can be formulated as follows:
    \begin{equation}
        {\rm Precision_{macro}}=\frac{1}{n} \sum_{k=1}^K \frac{TP_k}{TP_k+FP_k}
    \end{equation}
    \begin{equation}
        {\rm Recall_{macro}}=\frac{1}{n} \sum_{k=1}^K \frac{TP_k}{TP_k+FN_k}
    \end{equation}
    \begin{equation}
        {\rm F1_{macro}} = 2 \cdot \frac{{\rm Precision_{macro}} \cdot {\rm Recall_{macro}}}{{\rm Precision_{macro}} + {\rm Recall_{macro}}}
    \end{equation}
    \noindent The two tasks, \ie CHIP-CTC and KUAKE-QIC, adopt Macro-F1.

    \item \textbf{RougeL}. RougeL~\cite{lin2004automatic} has been widely used in machine translation and automatic text abstraction, which can measure the similarity between generated and ground-truth texts. Let $y$ and $\hat{y}$ denote the ground truth and generated texts, and their length are $m$ and $n$ respectively. Then, the RougeL can be formulated as:
    \begin{equation}
        R=\frac{{\rm LCS}(y, \hat{y})}{m}, P=\frac{{\rm LCS}(y, \hat{y})}{n}
    \end{equation}
    \begin{equation}
        {\rm RougeL}=\frac{(1+\beta^2\cdot R \cdot P)}{R+\beta^2 \cdot P}
    \end{equation}
    \noindent where ${\rm LCS}(\cdot,\cdot)$ computes the length of longest common subsequence. In the experiments, IMCS-V2-MRG and MedDG, as the text generation tasks, use this metric.
\end{itemize}

\section{Dataset} \label{sec:appendix_dataset}

In this section, we refer to more details about the dataset. The medical task descriptions and the prompt templates used for LLMs are shown in Table~\ref{tab:appendix_prompt}. From the description, we can find that the medical tasks are in large difference. Some tasks aim to extract informative entities or normalized clinical words, while others focus on the patient-doctor conversation. It verifies the task variety problem in real-world medical scenarios. 

As mentioned in Section~\ref{sec:preliminary_llm}, the original input and output of medical tasks are modified for using LLMs. We list out the prompt template examples of the dataset in Table~\ref{tab:appendix_prompt}. In the templates, ``[INPUT\_TEXT]'' represents the placeholder for medical texts. The medical texts vary with the different tasks. For example, the clinical report is inserted for CHIP-CDEE, whereas the doctor-patient conversations are used in MedDG and IMCS-V2-MRG tasks. ``[LIST\_LABELS]'' and ``[LIST\_MENTIONS]'' often refer to the task related candidates. For instance, the ``[LIST\_LABELS]'' in the CHIP-CDN task is replaced by several ICD-10 diagnosis words, which can assist the LLMs in generating correct answers. Only one template example for each task is listed due to the limited space, however, multiple templates actually exist and are used in the experiments for a better generalization~\cite{zhang2023instruction}.
